# Supplementary material for: Binarized Convolutional Neural Networks with Separable Filters for Efficient Hardware Acceleration
Source: arXiv:1707.04693 source file (2017-07-15)
Supplement: Supplementary file 1 [file supplementary.tex]

\subsection{Training on MNIST and SVHN}
%%% Topic: Learning curves on MNIST and SVHN

\begin{figure}[h]
	\centering
	\includegraphics[width=1.0\columnwidth]{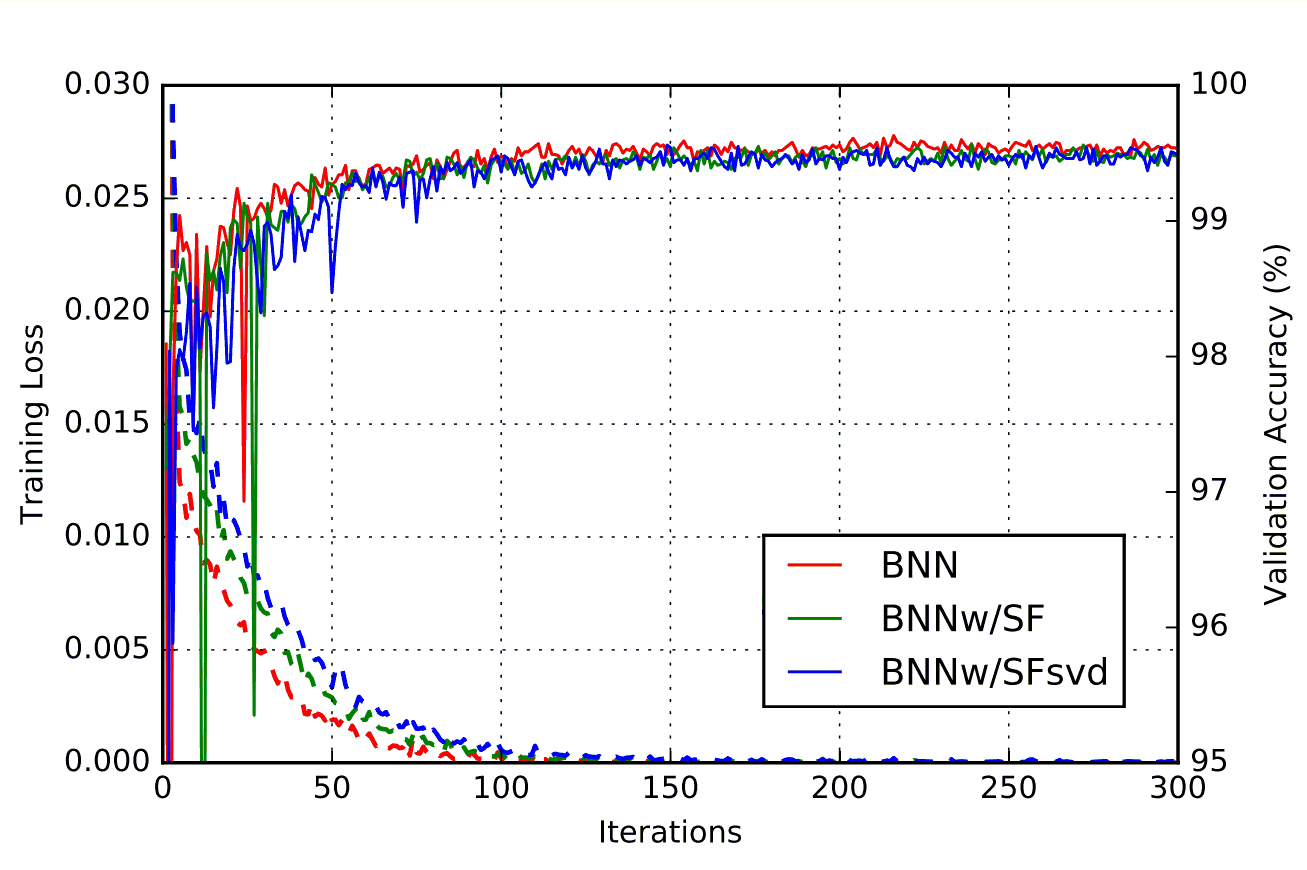}
	\caption{Learning Curves of ConvNets for BCNN(red), BCNNw/SF1(green) and BCNNw/SF2(blue) on MNIST dataset.
    The dotted lines represent the training costs(square hinge losses) and the continuous lines the corresponding validation error rates.}
   	\label{fig:learning_curve_mnist}
\end{figure}
Fig.~\ref{fig:learning_curve_mnist} shows the learning curves of BCNN and our training methods on MNIST.
Since the task of MNIST dataset is relatively easier than the other two datasets, our methods achieve almost the same accuracy as BCNN does.
% There are obvious differences in training loss because both of our two methods change the descending trajectories to a local minimum in the hypothesis space.
% It is clear to understand the reason why our method 1 has greater loss than that of BinaryNet due to a more aggressive noise.
% The loss difference between method 1 and method 2 is because the exact gradient over SVD limit descent to follow the exact gradient direction and magnitude w.r.t. the real-valued filters, while the method 1 uses a gradient of loss w.r.t. binarized separable filters to update the real-valued filters.
% We will discuss in detail the benefit of using exact gradient over the rank-1 approximation in next sub-section.

\begin{figure}[h]
	\centering
 	\includegraphics[width=1.0\columnwidth]{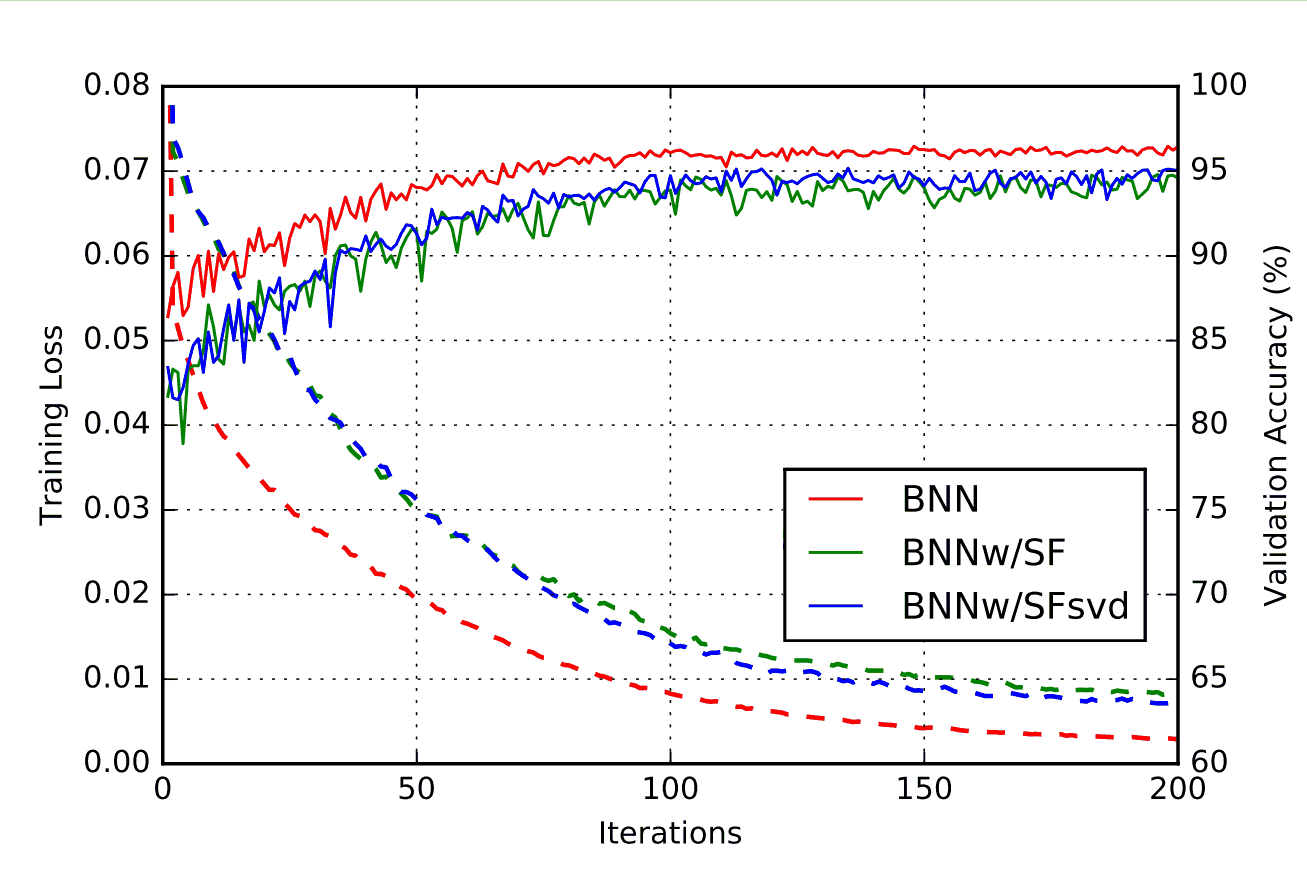}
	\caption{Learning Curves of ConvNets for BCNN(red), BCNNw/SF1(green) and BCNNw/SF2(blue) on SVHN dataset.
    The dotted lines represent the training costs(square hinge losses) and the continuous lines the corresponding validation error rates.}
    \label{fig:learning_curve_svhn}
\end{figure}
The learning curves on SVHN are shown in Fig.~\ref{fig:learning_curve_svhn}.
Although the task is to classify number digits as well, the diversity in real world is by far greater than that in MNIST dataset.
From the training loss we can see that simply to train $200$ epochs might be inadequate, and more epochs are suggested to get a better convergence in terms of training loss.
If we re-inspect Fig~\ref{fig:learning_curve_mnist} and~\ref{fig:learning_curve_cifar} again, the training loss in previous two datasets converge rapidly before the middle of entire training phase.
However, the diversity and three colorful channels hamper the learning of parameters.
One thing noteworthy is that our method 2 outperforms method 1 a little bit on SVHN.

\subsection{More Discussions on CIFAR-10}
%%% Topic: 1.
%%%		   2. filter frequencies for different layers

\begin{figure*}[h]
	\centering
 	\includegraphics[width=1.2\columnwidth]{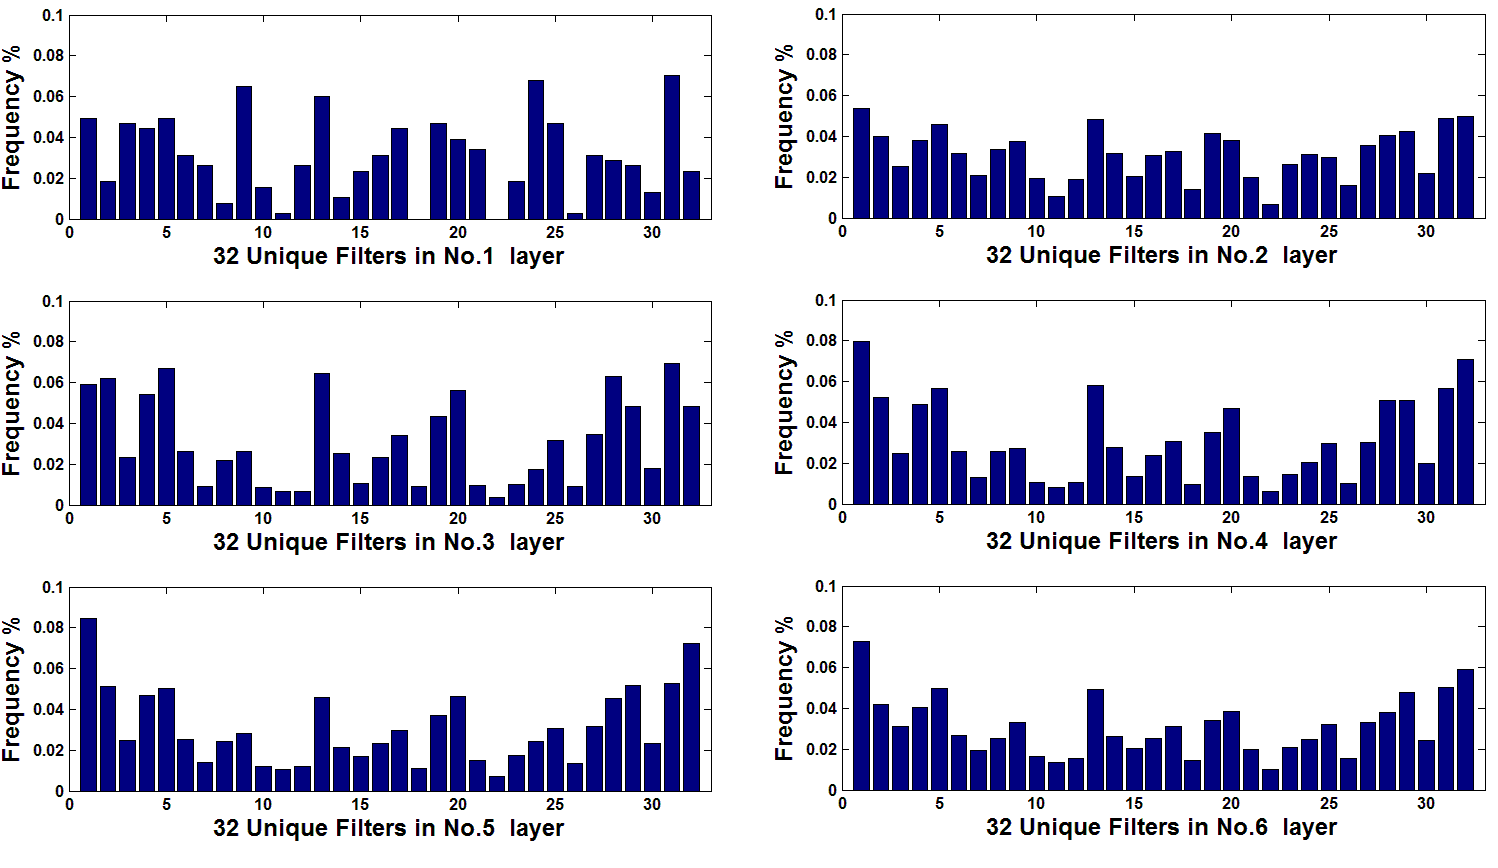}
	\caption{Unique Kernels Frequencies in Convolutional Layers}
    \label{fig:Frequency_6_layer}
\end{figure*}

\begin{figure}[h]
	\centering
 	\includegraphics[width=0.6\columnwidth]{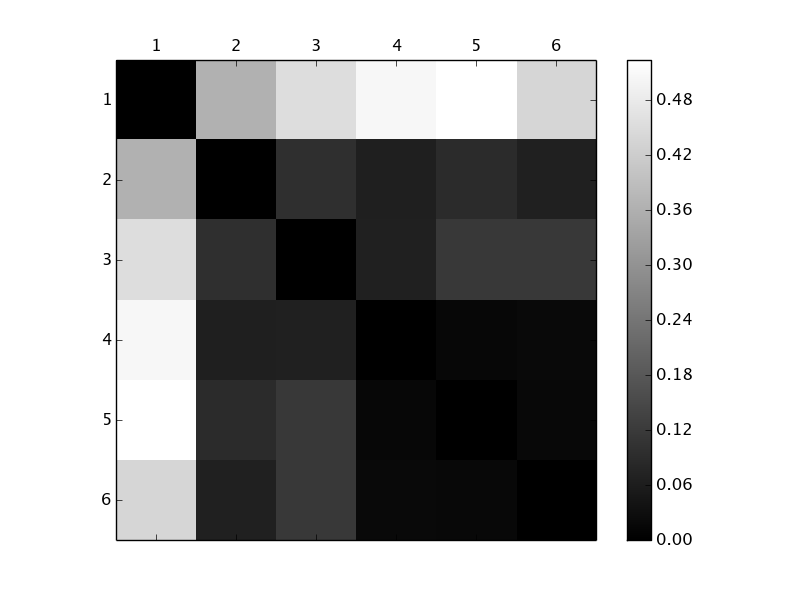}
	\caption{Pearson correlations among the six filter distributions. Every square stands for a distance between a pair of distributions.}
    \label{fig:pearson}
\end{figure}

Fig.~\ref{fig:Frequency_6_layer} shows the histograms of the trained filters on the six convolutional layers in our CIFAR-10 networks.
There are two important observations among the histograms:
\begin{itemize}
\item The relatively complicated filters, such as filter 11 and 22 in Fig.~\ref{fig:filter_draw}, are less preferred by the trained networks. Simpler filters with all black color, all white color or a strip are more likely to be preferred.
\item The histograms of layer 2, 4, and 6 are similar to each other, although differ in magnitude.
\end{itemize}
Fig.~\ref{fig:pearson} shows the correlations among the six filter distributions of the six convolutional layers, in which the darker the color is, the similar the pair of distributions are.
From the second row, we can see that the distributions on layer 2, 4, and 6 are similar with each other.
That means in the trained network, layer 2, 4, and 6 play similar role in the network.

\subsection{Larger Networks}
%%% Topic: 1. Explore larger models,
%%%		   2. Comparison on 5 CIFAR-10 mode

We also explore different sizes of networks for higher accuracy.
Tab.~\ref{tab:archi_bigger} lists two additional larger models for CIFAR-10.
The wider one stands for a model with all numbers of kernels doubled, and the deeper one is a network including two extra convolutional layers.
\begin{table*}[h]
\centering
\begin{tabular}{|c"c|c|c|}
\hline
Name       & Original    & Deeper       & Wider       \\ \thickhline
Input      & 3x32x32     & 3x32x32      & 3x32x32    \\ \hline
Conv-1     & 128x3x3x3   & 128x3x3x3   & 256x3x3x3    \\
Conv-2     & 128x128x3x3 & 128x128x3x3 & 256x256x3x3   \\ \hline
Pooling    & \multicolumn{3}{c|}{2 x 2 Max Pooling}  \\ \hline
Conv-3     & 256x128x3x3 & 256x128x3x3 & 512x256x3x3  \\
Conv-4     & 256x256x3x3 & 256x256x3x3 & 512x512x3x3 \\ \hline
Pooling    & \multicolumn{3}{c|}{2 x 2 Max Pooling}  \\ \hline
Conv-5     & 512x256x3x3 & 512x256x3x3 & 1024x512x3x3 \\
Conv-6     & 512x512x3x3 & 512x512x3x3 & 1024x1024x3x3 \\ \hline
Pooling    & \multicolumn{3}{c|}{2 x 2 Max Pooling}  \\ \hline
Conv-7     & - 			 & 512x512x3x3 & -           \\
Conv-8     & - 			 & 512x512x3x3 & -           \\ \hline
Pooling    & -           & 2 x 2 Max Pooling & -    \\ \hline
FC-1       & 1024x8192   & 1024x4096 & 1024x16,384  \\ \hline
FC-2       & 1024x1204   & 1024x1204   & 1024x1024   \\ \hline
FC-3       & 10x1024     & 10x1024     & 10x1024     \\ \hline
\end{tabular}
\vspace{0.2cm}
\caption{Besides the first column, which is the original model for CIFAR-10, column 2 shows a deeper model with two extra convolutional layers, and column 3 shows a widened network with all numbers of kernels doubled.}
\label{tab:archi_bigger}
\end{table*}

\begin{figure*}[hp]
	\centering
 	\includegraphics[width=1.2\columnwidth]{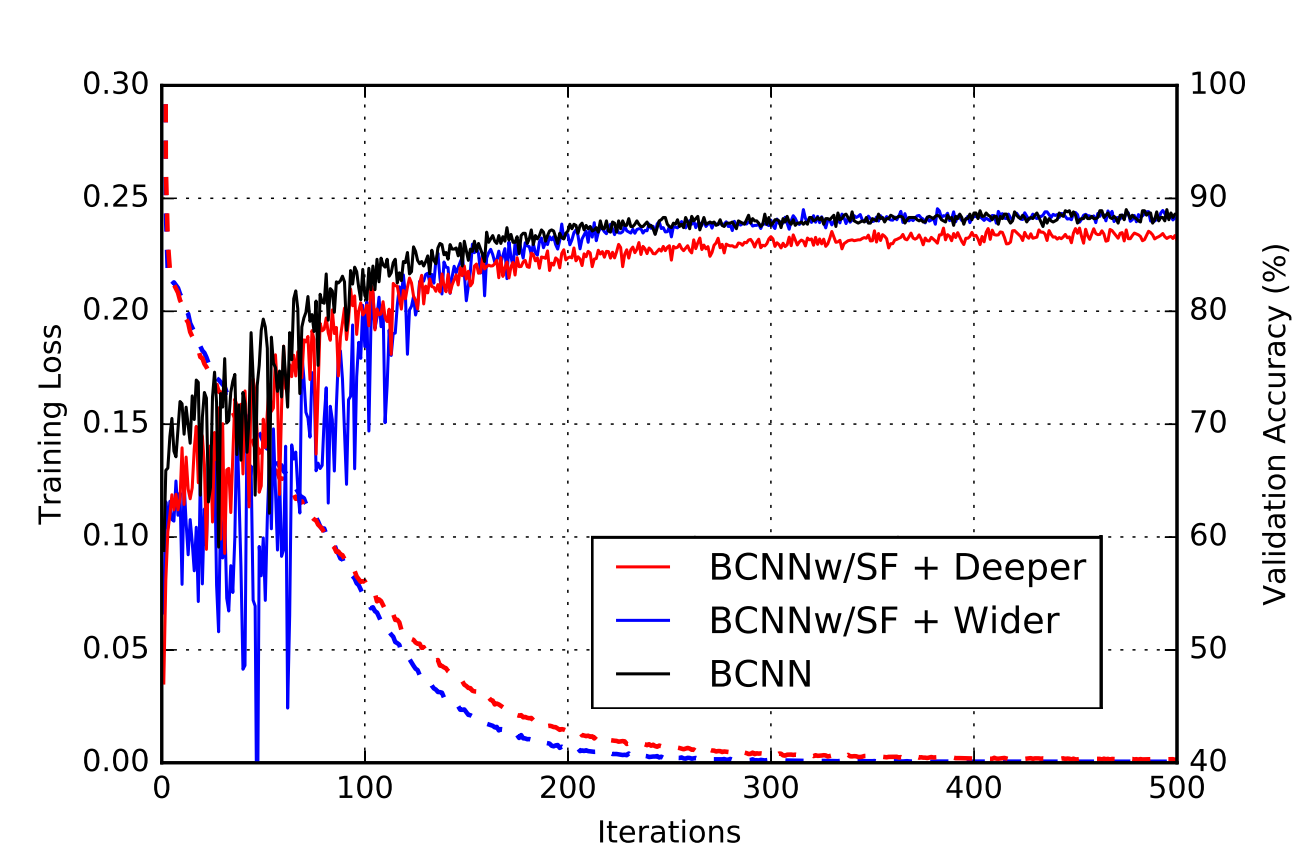}
	\caption{Learning Curves of ConvNets for BCNNw/SF with deeper Network(red), BCNNw/SF with wider Network(blue) and original BCNN on CIFAR-10 dataset.
    The dotted lines represent the training costs(square hinge losses) and the continuous lines the corresponding validation error rates.}
    \label{fig:learning_curve_all_500_cifar}
\end{figure*}
We train the two bigger networks with our method 1, and Fig.~\ref{fig:learning_curve_all_500_cifar} shows the learning curves of the two enlarged models for CIFAR-10.
Since the number of trainable parameters has been increased, it requires more epochs to travel in the hypothesis space and reach a local minimum.
Therefore, we train these two bigger networks with $500$ epochs, and compare with BCNN(BinaryNet).
As shown in Fig.~\ref{fig:learning_curve_all_500_cifar} the wider one (blue) starts with largest ripple yet catch up the same performance as BCNN(black) does around the 175th epoch.

\begin{table}[t]
\centering
\begin{tabular}{|l"c|}
\hline
Dataset                       & CIFAR-10 \\ \thickhline
BCNN(BinaryNet)~\cite{hubara2016bnn}	  & 11.40\%  \\ \hline
\multicolumn{2}{|c|}{Binarized Network with Separable Filters} \\ \hline
BCNNw/SF1 (this work)         & 14.12\%  \\ \hline
BCNNw/SF2 (this work)         & 15.46\%  \\ \hline
BCNNw/SF1 depper (this work)  & 14.11\%  \\ \hline
BCNNw/SF1 wider (this work)   & \textbf{11.68\%}  \\ \hline
\end{tabular}
\vspace{0.2cm}
\caption{Classification Accuracy (Error Rate) Comparison  on Different Datasets.
BCNNw/SF1 stands for our training method 1; BCNNw/SF2 denotes for our training method 2.}
\label{tab:results_bigger}
\end{table}
Tab.~\ref{tab:results_bigger} lists the results on CIFAR-10 of the two bigger models as well as the CIFAR-10 results in Tab.~\ref{tab:results}.
The performance improvement of deeper network is very scarce since the feature maps experience the extra destructive max pooling layer as shown in Tab.~\ref{tab:archi_bigger}, which reduces the size of the first fully-connected layer, FC-1, and hence suppresses the improvement.
The wider network achieves $11.68\%$, which is very close to the performance of BCNN(BinaryNet).
In summary, the accuracy degradation of BCNNw/SF can be compensated by enlarging the size of network.

\clearpage
